# Supplementary material for: Are We on the Same Page? Examining Developer Perception Alignment in Open Source Code Reviews
Source: arXiv:2504.18407 source file (2025-04-25)
Supplement: Supplementary file 1 [file appendix.tex]

\section{Codes from Open Coding}
\subsection{Objectives of Code Review}
\textbf{Question:} \textit{In your opinion, what are the most important objectives of the code review process?} 

% \textbf{Response:} A total of 14 codes were identified through the open coding process of the responses to this question. The table below provides a detailed breakdown of the codes, their definitions, and the percentage of participants who referenced each code in their responses. This data is presented separately for Contributors and Maintainers, along with the rank of each code based on the frequency of responses.

\begin{table*}[h]
    \centering
    \caption{Responses to perceived objectives of the code review process}

    \begin{tabular}{|l|l|}
        \hline
        \textbf{\textit{Code}} & \textbf{\textit{Definition}} \\ 
        \hline
        Community Building & The importance of fostering collaboration and a sense of community within the project \\
        \hline
        Conciseness & The need for code to be concise and free of unnecessary complexity\\
        \hline
        Correctness & Ensuring that the code works as intended and produces the correct outputs\\
        \hline
        Documentation & The importance of clear and comprehensive documentation for understanding the code\\
        \hline
        Functionality & Verifying that the code adds or enhances the intended functionality\\
        \hline
        Knowledge Sharing & Facilitating the transfer of knowledge and best practices through code reviews \\
        \hline
        Maintainability & Ensuring that the code is easy to maintain and adapt in the future \\
        \hline
        Motivation & Encouraging contributors and maintaining their motivation through positive feedback \\
        \hline
        Project Goal & Aligning the code changes with the overall goals of the project \\
        \hline
        Quality & Ensuring high-quality code that meets the project's standards \\
        \hline
        Security & Ensuring that the code adheres to security best practices \\
        \hline
        Standard & Adhering to coding standards and guidelines \\
        \hline
        Timeliness & Completing the code review process in a timely manner \\
        \hline
        Miscellaneous & Other minor factors mentioned by respondents\\
        \hline
    \end{tabular}
    \label{tab:objectives_details}
\end{table*}

\subsection{Key Factors for Contribution Approval}
\textbf{Question:} \textit{What do you believe are the key factors that ensure a contribution is approved during the code review process?}

% \textbf{Response:} This question resulted in the identification of several key factors that respondents believe are crucial for the approval of contributions during the code review process. The table below outlines these factors, along with their definitions, the percentage of participants who cited them, and their rank based on the frequency of responses.

\begin{table*}[h]
    \centering
        \caption{Responses to perceived key factors that ensure a contribution is accepted in the code review process}
        \begin{tabular}{|p{3cm}|p{11cm}|}
        \hline
        \textbf{\textit{Code}} & \textbf{\textit{Definition}}\\ 
        \hline
        Communication & Clear and effective communication between contributors and reviewers\\
        \hline
        Concise & How concise the contribution is\\
        \hline
        Correctness & The correctness of the contribution, ensuring it functions as expected including not introducing any bugs \\
        \hline
        Documentation & The inclusion of proper documentation with the contribution\\
        \hline
        Familiarity & The contributor's familiarity with the codebase and project \\
        \hline
        Good Intention & The perceived good intention behind the contribution \\
        \hline
        Maintainability & Ensuring that the contribution is maintainable in the long term \\
        \hline
        Novelty & The originality and innovativeness of the contribution \\
        \hline
        Project Goal & Alignment of the contribution with the overall project goals \\
        \hline
        Quality & The overall quality and adherence to project standards \\
        \hline
        Rationale & The rationale behind the contribution and its necessity \\
        \hline
        Responsiveness & The contributor's responsiveness to feedback during the review\\
        \hline
        Security & Consideration of security aspects in the contribution\\
        \hline
        Standard & Adherence to coding standards and guidelines \\
        \hline
        Timeliness & The timeliness of the contribution and review process \\
        \hline
        Understanding & The maintainer's of the code\\
        \hline
    \end{tabular}
    \label{tab:factors_details}
\end{table*}

\subsection{Witnessed bias}
\textbf{Question:} [If you ever noticed bias in the code review process], could you present the instance and how it was resolved

\textbf{Response:} Table \ref{tab:code_bias}
\begin{table}[h]
    \centering
    \caption{Definitions of codes to the responses about witnessed bias in the review process}
        \begin{tabular}{|p{3cm}|p{13cm}|}
            \hline
            \textbf{Code} & \textbf{Definition} \\ \hline
            Approach Difference & Bias resulting from differences in technical approaches or preferences between the reviewer and the author. \\ \hline
            Delay & Instances where the bias led to unnecessary delays in the review process. \\ \hline
            Other & Bias-related situations that did not fit into specific categories but were still noted. \\ \hline
            Proof it again & A situation where the reviewer insisted on rechecking code without sufficient reason, possibly due to bias. \\ \hline
            Familiarity Bias & Bias that occurred when the reviewer favored or was lenient towards familiar colleagues or their work. \\ \hline
            Discussion & Cases where bias was resolved through discussions between the reviewer and author. \\ \hline
            Misunderstanding & Instances where bias was the result of miscommunication or misunderstanding. \\ \hline
            More Reviewers & The recommendation or action of involving more reviewers to mitigate bias. \\ \hline
            Priority Bias & Bias caused by prioritizing certain tasks or individuals over others based on personal preferences. \\ \hline
            External Influence & Bias stemming from external factors influencing the review process, such as company culture or policies. \\ \hline
            Language Challenges & Bias arising from difficulties in communication due to language differences. \\ \hline
            Not adhering to Standard & Bias resulting from inconsistencies in adhering to agreed-upon coding or review standards. \\ \hline
            Social Pressure & Bias caused by peer pressure or social expectations within the team. \\ \hline
            Cultural Differences & Bias due to cultural misunderstandings or differences in working styles. \\ \hline
            Lack of Experience & Bias that arose from the inexperience of the reviewer or author, leading to an unbalanced review process. \\ \hline
            Personality Difference & Bias related to differences in personality or interpersonal conflicts. \\ \hline
            Prejudice & Explicit prejudice or discrimination based on personal attributes like race, gender, or background. \\ \hline
        \end{tabular}
    \label{tab:code_bias}
\end{table}
\subsection{Challenges in Code review}
\textbf{Question:} What are the challenges you face in implementing a code review process ?

\textbf{Response:} Table \ref{tab:code_challenges}

\begin{table}[h]
    \centering
    \caption{Definitions of Challenges in the OSS Code Review Process}
        \begin{tabular}{|p{4cm}|p{13cm}|}
            \hline
            \textbf{Code} & \textbf{Definition} \\ \hline
            Reviewer Responsiveness & Refers to the speed and effectiveness with which reviewers respond to code submissions. \\ \hline
            Communication Issues & Highlights the problems in communication between contributors and reviewers that affect the code review process. \\ \hline
            Lack of Documentation & Indicates insufficient or unclear documentation that makes it difficult for contributors to understand the code review process. \\ \hline
            Inconsistent Reviewer Experience & Refers to variability in the quality and thoroughness of code reviews depending on the reviewer. \\ \hline
            Volume & Refers to the high amount of code submissions that reviewers need to handle, which can be overwhelming. \\ \hline
            Unclear Expectations & Points to situations where contributors are unsure of what is expected from their code submissions during review. \\ \hline
            Code Quality Concerns & Refers to issues related to the perceived quality of the code being reviewed. \\ \hline
            Expectation Misalignment & Indicates a mismatch between what contributors submit and what reviewers expect in terms of standards or guidelines. \\ \hline
            Miscellaneous & Covers a variety of smaller, specific challenges that do not fit into the main categories but are still significant. \\ \hline
            Insufficient Effort & Refers to contributions that are perceived to be incomplete or maintainers believe demonstrate lack of effort from contributors to make them complete. \\ \hline
            Bias & Indicates the presence of conscious or unconscious biases in the code review process. \\ \hline
            Contributor Responsiveness & Refers to the speed and effectiveness with which contributors respond to feedback from reviewers. \\ \hline
            Tooling & Refers to the challenges associated with the tools used in the code review process. \\ \hline
            Over Complication & Points to the unnecessary complexity in the code review process that can hinder its efficiency. \\ \hline
        \end{tabular}
    \label{tab:code_challenges}
\end{table}

\subsection{Suggestions about the code review}
\textbf{Question:} What changes or improvements would you suggest for the code review process?

\textbf{Response:} Table \ref{tab:code_suggestions}
\begin{table}[h!]
    \centering
    \caption{Definitions of codes to the responses about suggestions for the review process}
        \begin{tabular}{|p{3cm}|p{13cm}|}
            \hline
            \textbf{Code} & \textbf{Definition} \\ \hline
            Improved Documentation & Recommendations related to enhancing the documentation to make code reviews more efficient and clear. \\ \hline
            Better Tools and Automation & Suggestions to introduce or improve the tools and automation used during the review process to streamline workflows. \\ \hline
            More Engagement & Requests for higher engagement from reviewers and participants in the code review process, ensuring active contributions. \\ \hline
            Enhanced Communication & Recommendations for improving the communication between team members during the review process to minimize misunderstandings. \\ \hline
            Enhanced Collaboration & Suggestions to encourage better collaboration among developers, fostering a more cooperative review environment. \\ \hline
            Improved Timeliness & Proposals to reduce delays and ensure the code review process is conducted in a timely manner. \\ \hline
            Miscellaneous & Other suggestions that did not fit into the main categories but are still valuable for improving the code review process. \\ \hline
        \end{tabular}
    \label{tab:code_suggestions}
\end{table}
