# Supplementary material for: Are We on the Same Page? Examining Developer Perception Alignment in Open Source Code Reviews
Source: arXiv:2504.18407 source file (2025-04-25)
Supplement: Supplementary file 2 [file appendix_data_tables.tex]

\section{Detailed Data Tables} \label{sec:data_tables}

\subsection{Perception of Guidelines and Process}
\textbf{Question:} How do the different groups perceive the accessibility and effectiveness of project guidelines toward addressing bias and promoting diversity and inclusiveness ?

\textbf{Response:} The data, as presented in Table \ref{tab:documents_and_process_details}, reveals distinct differences in the perception of project guidelines between Contributors and Maintainers.
\begin{table*}[h]
    \centering
    \resizebox{\textwidth}{!}{
        \begin{tabular}{|p{10cm}|p{0.6cm}|p{0.7cm}|p{0.7cm}|p{0.7cm}|p{0.7cm}|p{0.7cm}|p{0.7cm}|p{0.7cm}|p{0.7cm}|p{0.7cm}|p{0.7cm}|p{0.7cm}|}
        \hline
        \multirow{2}{*}{\textbf{}} & \multicolumn{6}{c|}{\textbf{Contributors}} & \multicolumn{6}{c|}{\textbf{Maintainers}} \\
        \cline{2-13}
        & \centering \textbf{SD} & \centering \textbf{D} & \centering \textbf{N} & \centering \textbf{A} & \centering \textbf{SA} & \centering \textbf{NA} & \centering \textbf{SD} & \centering \textbf{D} & \centering \textbf{N} & \centering \textbf{A} & \centering \textbf{SA} & \textbf{NA} \\
        \hline
        Guideline for code review process are sufficiently documented  & 2.26\% & 11.30\% & 20.34\% & 40.68\% & 18.64\% & 6.78\% & 3.85\% & 7.69\% & 13.46\% & 46.15\% & 25.00\% & 3.85\% \\
        \hline
        Documents are easily accessible to contributors  & 3.39\% & 5.08\% & 12.43\% & 36.16\% & 35.03\% & 7.91\% & 1.92\% & 7.69\% & 3.85\% & 44.23\% & 38.46\% & 3.85\% \\
        \hline
        Documents clearly describe the expectation from me while I perform my code review task  & 2.84\% & 8.52\% & 22.73\% & 36.93\% & 17.61\% & 11.36\% & 0.00\% & 9.62\% & 19.23\% & 44.23\% & 19.23\% & 7.69\% \\
        \hline
        Documents have effectively addressed bias in the code review process & 4.55\% & 15.91\% & 34.09\% & 19.32\% & 7.95\% & 18.18\% & 5.77\% & 13.46\% & 40.38\% & 21.15\% & 7.69\% & 11.54\% \\
        \hline
        Documents have clearly defined the process to mitigate bias in the code review process & 3.98\% & 20.45\% & 33.52\% & 21.02\% & 5.11\% & 15.91\% & 3.85\% & 15.38\% & 42.31\% & 23.08\% & 5.77\% & 9.62\% \\
        \hline
        Documents have clearly defined the standard for communication during code review process to minimize conflict & 5.71\% & 8.00\% & 28.00\% & 29.71\% & 17.14\% & 11.43\% & 1.92\% & 17.31\% & 17.31\% & 40.38\% & 15.38\% & 7.69\% \\
        \hline
        Objectives of the code review process as presented in these documentations are inline with my expectation for code review & 2.27\% & 7.95\% & 23.30\% & 31.25\% & 23.30\% & 11.93\% & 0.00\% & 1.92\% & 15.38\% & 51.92\% & 21.15\% & 9.62\% \\
        \hline
        \multicolumn{13}{|l|}{\textbf{Current Code Review Process}} \\
        \hline
        Improves software quality & 1.14\% & 1.70\% & 9.66\% & 51.70\% & 35.80\% & - & 3.06\% & 1.02\% & 6.12\% & 48.98\% & 40.82\% & - \\
        \hline
        Effectively mitigates bias & 1.70\% & 12.50\% & 47.73\% & 31.25\% & 6.82\% & - & 7.14\% & 9.18\% & 41.84\% & 33.67\% & 8.16\% & - \\
        \hline
        Promotes diversity and inclusivity & 5.11\% & 10.80\% & 46.02\% & 27.84\% & 10.23\% & - & 10.20\% & 12.24\% & 38.78\% & 23.47\% & 15.31\% & - \\
        \hline
        Follows standard for communication during code review process to minimize conflict & 1.70\% & 6.82\% & 24.43\% & 50.00\% & 17.05\% & - & 6.12\% & 6.12\% & 24.49\% & 44.90\% & 18.37\% & - \\
        \hline
        \end{tabular}}
    \caption{Detailed data on project perception of guidelines and process}
    \label{tab:documents_and_process_details}
\end{table*}

\begin{center}
    \textbf{Table \ref{tab:documents_and_process_details} Keys:} SD = Strongly Disagree, D = Disagree, N = Neutral, A = Agree, SA = Strongly Agree, NA = Not Applicable
\end{center}

\begin{table}[h]
    \centering
    \resizebox{\textwidth}{!}{
        \begin{tabular}{|l|p{16cm}|}
            \hline
            \textbf{Suggestion} & \textbf{Definition} \\ \hline
            Better Tools and Automation & Suggests the implementation of improved tools and automation to streamline and facilitate the code review process. \\ \hline
            Improved Documentation & Advocates for better and more comprehensive documentation to help contributors understand the code review process and requirements. \\ \hline
            Enhanced Communication & Recommends improving communication between contributors and reviewers to ensure clarity and mutual understanding. \\ \hline
            Enhanced Collaboration & Suggests fostering greater collaboration among contributors and reviewers to improve the quality and efficiency of code reviews. \\ \hline
            More Engagement & Encourages more active participation and engagement from all parties involved in the code review process. \\ \hline
            Improved Timeliness & Emphasizes the need for faster turnaround times in the code review process to prevent delays in the development cycle. \\ \hline
            Miscellaneous & Includes various other suggestions that are not categorized under the main suggestions but are still relevant to improving the process. \\ \hline
        \end{tabular}
    }
    \caption{Definitions of Suggestions to Improve the OSS Code Review Process}
    \label{tab:oss_code_review_suggestions_definitions}
\end{table}

\subsection{Experience of Bias}
Participants were asked if they have experienced or noticed bias in the code review process. Their response is presented in Table \ref{tab:prevalence_of_bias} segmented by various demographic and professional categories, including age group, gender, education level, professional experience, and open source experience. The table shows the percentage of respondents within each category who answered "Yes" to the question, with separate columns for contributors, maintainers, and the overall group.

The youngest age group (18-24) has a relatively low percentage of maintainers who reported noticing bias (21.74\%) compared to contributors (34.29\%). However, in the overall category, a high percentage (70.69\%) reported noticing bias, indicating that younger individuals may be more sensitive to or aware of bias in general, even if they have less experience as maintainers.

In general, Males have a higher percentage of respondents who did not notice bias compared to females, especially among contributors (60.80\% of males versus 50.00\% of females). This could reflect differences in perception or experiences of bias between genders. The percentage of females who reported noticing bias is higher than males in both contributor and maintainer roles. For females, 50.00\% of contributors and 57.14\% of maintainers reported noticing bias. This could suggest that women are more likely to perceive or report bias in code reviews.

There is a substantial percentage difference between contributors and maintainers among Multiracial respondents, with 77.78\% of maintainers noticing bias compared to 33.33\% of contributors. This could indicate that multiracial individuals in leadership or reviewer roles are more likely to experience or identify bias. A significant portion of Asian respondents noticed bias, particularly among maintainers (37.93\%). This suggests that Asian individuals might be more likely to perceive bias in their work environments. The data for groups like Black or African American and Native American or Alaska Native is less consistent, with small sample sizes possibly affecting the reliability of the percentages. 

Respondents with higher education levels (Doctorate, Masters) generally reported noticing bias more frequently, particularly in the maintainer role. This may suggest that more educated individuals are either more aware of or more willing to report bias. There is a noticeable variability in the responses from those with high school and associate degrees, which might reflect less consistent experiences or perceptions of bias within these groups.

Those with less professional experience tend to report noticing bias more frequently, especially among maintainers (37.50\%). This could suggest that less experienced individuals are more sensitive to bias or that their early experiences in the field are more impacted by it. Among those with over 10 years of experience, the percentages are more balanced, but there is still a considerable percentage (44.00\% of contributors) reporting bias, which indicates that bias perception doesn’t necessarily diminish with experience. Similarly, respondents with less than a year of open source experience reported a high rate of bias (76.19\% overall), especially in the maintainer role, which may indicate that those new to open source are more likely to encounter or perceive bias.

Younger, less experienced, and female respondents tend to report noticing bias more frequently. Racial/ethnic differences show that certain groups, particularly Multiracial respondents, perceive more bias when in roles of authority (like maintainers). Higher levels of education correlate with a greater perception of bias, potentially due to increased awareness or willingness to report it. Experience in open source also plays a role, with newer contributors reporting more bias than those with extensive experience.

\begin{table}[htbp!]
    \centering
    \resizebox{0.95\textwidth}{!}{
        \begin{tabular}{|l|l|c|c|c|}
            \cline{1-5}
            \multicolumn{2}{|c|}{\textbf{Group}} & \textbf{Contributors} & \textbf{Maintainers} & \textbf{All} \\
            \cline{3-5}
            \cline{1-5}
            \multirow{6}{*}{\rotatebox{90}{\parbox{2cm}{\centering Age Group}}} 
                & 18-24 (58) & 34.29\% & 21.74\% & 70.69\% \\
                \cline{2-5}
                & 25-34 (143) & 41.57\% & 46.30\% & 56.64\% \\
                \cline{2-5}
                & 35-44 (61) & 47.73\% & 58.82\% & 49.18\% \\
                \cline{2-5}
                & 45-54 (20) & 27.27\% & 44.44\% & 65.00\% \\
                \cline{2-5}
                & 55-64 (7) & 28.57\% & 0.00\% & 71.43\% \\
                \cline{2-5}
                & 64-above (1) & 0.00\% & 0.00\% & 100.00\% \\
                \cline{1-5}
            \multirow{4}{*}{\rotatebox{90}{\centering Gender}}
                & Female (11) & 50.00\% & 57.14\% & 45.45\% \\
                \cline{2-5}
                & Male (270) & 39.20\% & 41.49\% & 60.00\% \\
                \cline{2-5}
                & Non-binary/Third gender (4) & 50.00\% & 0.00\% & 50.00\% \\
                \cline{2-5}
                & Prefer not to say (5) & 66.67\% & 50.00\% & 40.00\% \\
                \cline{1-5}
            \multirow{8}{*}{\rotatebox{90}{\parbox{3.25cm}{\centering Racial/Ethnic Group}}}
                & Asian (86) & 36.84\% & 37.93\% & 62.79\% \\
                \cline{2-5}
                & Black or African American (2) & 50.00\% & 0.00\% & 50.00\% \\
                \cline{2-5}
                & Multiracial (24) & 33.33\% & 77.78\% & 50.00\% \\
                \cline{2-5}
                & Native American or Alaska Native (15) & 15.38\% & 100.00\% & 73.33\% \\
                \cline{2-5}
                & Native Hawaiian or Other Pacific Islander (1) & 100.00\% & 0.00\% & 0.00\% \\
                \cline{2-5}
                & Other (12) & 44.44\% & 66.67\% & 50.00\% \\
                \cline{2-5}
                & Prefer not to say (143) & 45.35\% & 38.60\% & 57.34\% \\
                \cline{2-5}
                & White (7) & 50.00\% & 0.00\% & 71.43\% \\
                \cline{1-5}
            \multirow{6}{*}{\rotatebox{90}{\parbox{2cm}{\centering Education Level}}} 
                & Associates (8) & 28.57\% & 100.00\% & 62.50\% \\
                \cline{2-5}
                & Bachelors (133) & 33.77\% & 46.43\% & 60.90\% \\
                \cline{2-5}
                & College (24) & 60.00\% & 33.33\% & 50.00\% \\
                \cline{2-5}
                & Doctorate (17) & 33.33\% & 60.00\% & 58.82\% \\
                \cline{2-5}
                & High school (45) & 46.67\% & 40.00\% & 55.56\% \\
                \cline{2-5}
                & Masters (63) & 43.48\% & 29.41\% & 60.32\% \\
                \cline{1-5}
            \multirow{5}{*}{\rotatebox{90}{\parbox{1.75cm}{\centering Professional Exp.}}}
                & <1 (15) & 28.57\% & 37.50\% & 66.67\% \\
                \cline{2-5}
                & 1-3 (52) & 17.14\% & 23.53\% & 80.77\% \\
                \cline{2-5}
                & 4-6 (62) & 43.24\% & 48.00\% & 54.84\% \\
                \cline{2-5}
                & 7-10 (54) & 54.55\% & 42.86\% & 50.00\% \\
                \cline{2-5}
                & 10< (107) & 44.00\% & 50.00\% & 54.21\% \\
                \cline{1-5}
            \multirow{5}{*}{\rotatebox{90}{\parbox{1.75cm}{\centering Open Source Exp.}}}
                & <1 (21) & 17.65\%  & 50.00\%  & 76.19\% \\
                \cline{2-5}
                & 1-3 (69) & 32.56\%  & 30.77\%  & 68.12\%  \\
                \cline{2-5}
                & 4-6 (86) & 43.75\%  & 36.84\%  & 59.30\%  \\
                \cline{2-5}
                & 7-10 (54) & 45.00\%  & 57.14\%  & 51.85\%  \\
                \cline{2-5}
                & 10< (60) & 48.72\%  & 57.14\%  & 48.33\%  \\
                \cline{1-5}
            \multicolumn{2}{|c|}{\textbf{All}} 
                & 40.11\%  & 42.72\%  & \\
            \cline{1-5}
        \end{tabular}
        }
        \caption{Percentage of respondents who reported noticing bias in the code review process, broken down by demographic attributes}
        \label{tab:prevalence_of_bias}
\end{table}

\subsection{Experience of Bias}
Participants were asked if they have experienced or noticed bias in the code review process. Their response is presented in Table \ref{tab:prevalence_of_bias} segmented by various demographic and professional categories, including age group, gender, education level, professional experience, and open source experience. The table shows the percentage of respondents within each category who answered "Yes" to the question, with separate columns for contributors, maintainers, and the overall group.

The youngest age group (18-24) has a relatively low percentage of maintainers who reported noticing bias (21.74\%) compared to contributors (34.29\%). However, in the overall category, a high percentage (70.69\%) reported noticing bias, indicating that younger individuals may be more sensitive to or aware of bias in general, even if they have less experience as maintainers.

In general, Males have a higher percentage of respondents who did not notice bias compared to females, especially among contributors (60.80\% of males versus 50.00\% of females). This could reflect differences in perception or experiences of bias between genders. The percentage of females who reported noticing bias is higher than males in both contributor and maintainer roles. For females, 50.00\% of contributors and 57.14\% of maintainers reported noticing bias. This could suggest that women are more likely to perceive or report bias in code reviews.

There is a substantial percentage difference between contributors and maintainers among Multiracial respondents, with 77.78\% of maintainers noticing bias compared to 33.33\% of contributors. This could indicate that multiracial individuals in leadership or reviewer roles are more likely to experience or identify bias. A significant portion of Asian respondents noticed bias, particularly among maintainers (37.93\%). This suggests that Asian individuals might be more likely to perceive bias in their work environments. The data for groups like Black or African American and Native American or Alaska Native is less consistent, with small sample sizes possibly affecting the reliability of the percentages. 

Respondents with higher education levels (Doctorate, Masters) generally reported noticing bias more frequently, particularly in the maintainer role. This may suggest that more educated individuals are either more aware of or more willing to report bias. There is a noticeable variability in the responses from those with high school and associate degrees, which might reflect less consistent experiences or perceptions of bias within these groups.

Those with less professional experience tend to report noticing bias more frequently, especially among maintainers (37.50\%). This could suggest that less experienced individuals are more sensitive to bias or that their early experiences in the field are more impacted by it. Among those with over 10 years of experience, the percentages are more balanced, but there is still a considerable percentage (44.00\% of contributors) reporting bias, which indicates that bias perception doesn’t necessarily diminish with experience. Similarly, respondents with less than a year of open source experience reported a high rate of bias (76.19\% overall), especially in the maintainer role, which may indicate that those new to open source are more likely to encounter or perceive bias.

Younger, less experienced, and female respondents tend to report noticing bias more frequently. Racial/ethnic differences show that certain groups, particularly Multiracial respondents, perceive more bias when in roles of authority (like maintainers). Higher levels of education correlate with a greater perception of bias, potentially due to increased awareness or willingness to report it. Experience in open source also plays a role, with newer contributors reporting more bias than those with extensive experience.

\begin{table}[htbp!]
    \centering
    \resizebox{0.95\textwidth}{!}{
        \begin{tabular}{|l|l|c|c|c|}
            \cline{1-5}
            \multicolumn{2}{|c|}{\textbf{Group}} & \textbf{Contributors} & \textbf{Maintainers} & \textbf{All} \\
            \cline{3-5}
            \cline{1-5}
            \multirow{6}{*}{\rotatebox{90}{\parbox{2cm}{\centering Age Group}}} 
                & 18-24 (58) & 34.29\% & 21.74\% & 70.69\% \\
                \cline{2-5}
                & 25-34 (143) & 41.57\% & 46.30\% & 56.64\% \\
                \cline{2-5}
                & 35-44 (61) & 47.73\% & 58.82\% & 49.18\% \\
                \cline{2-5}
                & 45-54 (20) & 27.27\% & 44.44\% & 65.00\% \\
                \cline{2-5}
                & 55-64 (7) & 28.57\% & 0.00\% & 71.43\% \\
                \cline{2-5}
                & 64-above (1) & 0.00\% & 0.00\% & 100.00\% \\
                \cline{1-5}
            \multirow{4}{*}{\rotatebox{90}{\centering Gender}}
                & Female (11) & 50.00\% & 57.14\% & 45.45\% \\
                \cline{2-5}
                & Male (270) & 39.20\% & 41.49\% & 60.00\% \\
                \cline{2-5}
                & Non-binary/Third gender (4) & 50.00\% & 0.00\% & 50.00\% \\
                \cline{2-5}
                & Prefer not to say (5) & 66.67\% & 50.00\% & 40.00\% \\
                \cline{1-5}
            \multirow{8}{*}{\rotatebox{90}{\parbox{3.25cm}{\centering Racial/Ethnic Group}}}
                & Asian (86) & 36.84\% & 37.93\% & 62.79\% \\
                \cline{2-5}
                & Black or African American (2) & 50.00\% & 0.00\% & 50.00\% \\
                \cline{2-5}
                & Multiracial (24) & 33.33\% & 77.78\% & 50.00\% \\
                \cline{2-5}
                & Native American or Alaska Native (15) & 15.38\% & 100.00\% & 73.33\% \\
                \cline{2-5}
                & Native Hawaiian or Other Pacific Islander (1) & 100.00\% & 0.00\% & 0.00\% \\
                \cline{2-5}
                & Other (12) & 44.44\% & 66.67\% & 50.00\% \\
                \cline{2-5}
                & Prefer not to say (143) & 45.35\% & 38.60\% & 57.34\% \\
                \cline{2-5}
                & White (7) & 50.00\% & 0.00\% & 71.43\% \\
                \cline{1-5}
            \multirow{6}{*}{\rotatebox{90}{\parbox{2cm}{\centering Education Level}}} 
                & Associates (8) & 28.57\% & 100.00\% & 62.50\% \\
                \cline{2-5}
                & Bachelors (133) & 33.77\% & 46.43\% & 60.90\% \\
                \cline{2-5}
                & College (24) & 60.00\% & 33.33\% & 50.00\% \\
                \cline{2-5}
                & Doctorate (17) & 33.33\% & 60.00\% & 58.82\% \\
                \cline{2-5}
                & High school (45) & 46.67\% & 40.00\% & 55.56\% \\
                \cline{2-5}
                & Masters (63) & 43.48\% & 29.41\% & 60.32\% \\
                \cline{1-5}
            \multirow{5}{*}{\rotatebox{90}{\parbox{1.75cm}{\centering Professional Exp.}}}
                & <1 (15) & 28.57\% & 37.50\% & 66.67\% \\
                \cline{2-5}
                & 1-3 (52) & 17.14\% & 23.53\% & 80.77\% \\
                \cline{2-5}
                & 4-6 (62) & 43.24\% & 48.00\% & 54.84\% \\
                \cline{2-5}
                & 7-10 (54) & 54.55\% & 42.86\% & 50.00\% \\
                \cline{2-5}
                & 10< (107) & 44.00\% & 50.00\% & 54.21\% \\
                \cline{1-5}
            \multirow{5}{*}{\rotatebox{90}{\parbox{1.75cm}{\centering Open Source Exp.}}}
                & <1 (21) & 17.65\%  & 50.00\%  & 76.19\% \\
                \cline{2-5}
                & 1-3 (69) & 32.56\%  & 30.77\%  & 68.12\%  \\
                \cline{2-5}
                & 4-6 (86) & 43.75\%  & 36.84\%  & 59.30\%  \\
                \cline{2-5}
                & 7-10 (54) & 45.00\%  & 57.14\%  & 51.85\%  \\
                \cline{2-5}
                & 10< (60) & 48.72\%  & 57.14\%  & 48.33\%  \\
                \cline{1-5}
            \multicolumn{2}{|c|}{\textbf{All}} 
                & 40.11\%  & 42.72\%  & \\
            \cline{1-5}
        \end{tabular}
        }
        \caption{Percentage of respondents who reported noticing bias in the code review process, broken down by demographic attributes}
        \label{tab:prevalence_of_bias}
\end{table}
