# Supplementary material for: Are We on the Same Page? Examining Developer Perception Alignment in Open Source Code Reviews
Source: arXiv:2504.18407 source file (2025-04-25)
Supplement: Supplementary file 3 [file appendix_interview_guide.tex]

\section*{Interview Guide} \label{sec:interview_guide}

\subsection*{Open Source Software (OSS) Code Review Process Interview}

\subsubsection*{Introduction}

My name is \_\_\{name\}\_\_. I am a graduate student at Virginia Tech, and I am conducting this interview as part of my research project. Thank you for taking the time to fill out the survey and signing up to provide additional information through this interview.

The core objective of this study is to delve into the code review mechanisms that are pivotal to the evolution and integrity of OSS. By gathering insights from both contributors and maintainers, we aim to paint a comprehensive picture of the current landscape, identify areas for improvement, and understand the tools and practices that can enhance the code review experience and mitigate biases. For this project, bias in code review is defined as any prejudicial treatment of contributions or contributors based on factors unrelated to the merit of the work, such as the contributor's identity, background, or the nature of the changes.

In this interview, you will be asked to discuss your experiences as a \_\_\{maintainer/contributor\}\_\_ on open source projects. Your responses will remain anonymous and will be used to explore ways to improve open source development and software engineering in general. The interview will take approximately 30-45 minutes. You may withdraw from this interview at any time without consequences and may also refuse to answer any questions you don’t want to answer while remaining in the study.

Any data collected during this interview will be kept confidential. Your interview will be recorded using Zoom. The recordings will be uploaded to a secure, password-protected computer and will only be accessible by the research team. We will transcribe and code the transcripts using an anonymous participant ID. Also, please do not use any names or identifying information about your colleagues in your responses.

Do you consent to participate in this interview?

If yes, continue.

\subsubsection*{Warm-up Question}
\begin{itemize}
    \item Can you briefly describe your background as a developer and how you got started with open source projects?
\end{itemize}

\subsubsection*{Main Questions}

\begin{enumerate}
    \item You listed \_\_\_\_ as one of the key factors to ensure approval of a contribution during the code review process. Could you elaborate?
    \begin{itemize}
        \item How often do you encounter situations where these factors were not considered, and the outcome was not favorable?
        \item Do you believe this is understood by both contributors and reviewers?
        \item Do the documents/guidelines for contribution reflect these factors clearly? If not, what do you suggest?
        \item How do you think the process could be improved based on this experience?
    \end{itemize}
    \item Can you share an example of how specific documentation or guidelines significantly influenced your approach to code review?
    \item Were there any discrepancies between your expectations and the actual process outlined in the documents?
    \item Do you believe the code review process is successful in addressing issues of bias? Can you provide specific instances where they failed?
    \begin{itemize}
        \item Follow-up on:
        \begin{itemize}
            \item Effectively mitigating bias
            \item Promoting diversity and inclusivity
            \item Following standards for communication during the code review process to minimize conflict
            \item How did this impact the project?
        \end{itemize}
    \end{itemize}
    \item In your opinion, what is required from the guidelines to mitigate bias?
    \item For participants who indicated they don’t use external resources, ask why.
    \item For participants who indicated they use external resources, ask how these external resources complement the existing project documentation on code review.
    \begin{itemize}
        \item Are there certain aspects or perspectives that you find only in external resources?
        \item Do these resources introduce any additional complexity to or detract from the process?
    \end{itemize}
    \item Can you detail a particularly challenging code review you participated in and how you navigated those challenges?
    \begin{itemize}
        \item What lessons were learned that could be applied to the code review process?
    \end{itemize}
    \item Can you provide an example of a time when you encountered a report of unnecessary pushback or bias towards someone’s contributions, and explain how it was resolved?
    \begin{itemize}
        \item Do you feel that the code review process and the guidelines helped in resolving this challenge?
    \end{itemize}
    \item You suggested \_\_\_\_ to improve the code review process. Could you elaborate?
\end{enumerate}

\subsection*{Conclusion}

\begin{itemize}
    \item Thank the interviewee for their time and insights.
    \item Ask if they have any questions or additional feedback to provide.
    \item Offer to share the findings or improvements made based on the interview.
\end{itemize}
