# Supplementary material for: Are We on the Same Page? Examining Developer Perception Alignment in Open Source Code Reviews
Source: arXiv:2504.18407 source file (2025-04-25)
Supplement: Supplementary file 4 [file appendix_survey_questions.tex]

\section{Contributor Survey Questions} \label{sec:contributor_survey}

\textbf{Welcome to the Open Source Software (OSS) Code Review Process Survey}
\subsection*{Introduction}
Thank you for your interest in participating in this survey. Your input is invaluable in advancing our understanding of code review processes within Open Source Software (OSS) projects. This research aims to explore the intricacies and expectations of individuals like yourself who contribute to the rich ecosystem of OSS. In this survey, we use the term "code review" to refer to any of the following: "pull request review," "merge request review," or "change request review."

\subsection*{Purpose of the Study}
The core objective of this study is to delve into the code review mechanisms that are pivotal to the evolution and integrity of OSS. By gathering insights from both contributors and maintainers, we aim to paint a comprehensive picture of the current landscape, identify areas for improvement, and understand the tools and practices that can enhance the code review experience and mitigate biases. Bias in code review refers to the prejudicial treatment of contributions or contributors based on factors unrelated to the merit of the work, such as the contributor's identity, background, or the nature of the changes.

\subsection*{Who Should Participate}
Please note that to engage in this survey, participants are required to be aged 18 years or older. This survey is designed for:

\begin{itemize}
    \item \textbf{Contributors}: Programmers who submit code changes to OSS projects for improvements, bug fixes, or new functionalities.
\end{itemize}

Your experiences and perceptions as a contributor or maintainer are crucial in shaping the outcomes of this research.

\subsection*{What to Expect in This Survey}
The following areas will be covered in the survey:
\begin{itemize}
    \item Your role and experience in OSS projects.
    \item Expectations and experiences with the code review process.
    \item The use of tools, guidelines, or materials in facilitating code review.
    \item Perspectives on how code review processes can be improved to reduce bias.
\end{itemize}
In addition to demographic and background questions, there are 12 core questions in this survey, and we expect it to take about 10-12 minutes to complete.

\subsection*{Confidentiality}
Your responses will be kept confidential, and the data will be analyzed in aggregate form anonymously. However, we cannot protect the data to GDPR standards.

\subsection*{Consent}
Your participation in this survey is voluntary. If any question makes you feel uncomfortable, you can simply stop participating or close the browser window. You may decide not to participate at all, or, if you start the study, you may withdraw at any time. By proceeding with this survey, you acknowledge that you have read and understood the purpose of the research and agree to participate voluntarily.

\subsection*{Contact Information}
Should you have any questions or require further information about the study, please contact \textbf{\textit{<redacted for review>.}}.

\subsection*{Start Survey}
To begin the survey, please click the "Start" button below. Thank you for your time and valuable contribution to this study.

\subsubsection*{Survey Questions}

\begin{enumerate}
    \item Please select your age group. *
    \begin{itemize}
        \item 18-24
        \item 25-34
        \item 35-44
        \item 45-54
        \item 55-64
        \item Above 64
    \end{itemize}
    \item Which of the following best describes your gender? *
    \begin{itemize}
        \item Male
        \item Female
        \item Non-binary/Third gender
        \item Prefer not to say
        \item Prefer to self-describe
    \end{itemize}
    \item What is the highest level of education you have completed? 
    \begin{itemize}
        \item High school diploma or equivalent
        \item Some college, no degree
        \item Associate degree
        \item Bachelor’s degree
        \item Master’s degree
        \item Doctorate or higher
    \end{itemize}
    \item Please select the race/ethnicity group(s) with which you most closely identify. (Select all that apply) *
    \begin{itemize}
        \item Asian
        \item Black or African American
        \item Hispanic or Latino
        \item Native American or Alaska Native
        \item Native Hawaiian or Other Pacific Islander
        \item Middle Eastern or North African
        \item Multiracial
        \item White
        \item Prefer not to say
        \item Other (please specify)
    \end{itemize}
    \item How many years of professional experience do you have in software development? *
    \begin{itemize}
        \item Less than 1 year
        \item 1-3 years
        \item 4-6 years
        \item 7-10 years
        \item More than 10 years
    \end{itemize}
    \item What best describes your current role in the open source project? *
    \begin{itemize}
        \item Developer/Engineer
        \item Team Lead/Manager
        \item Quality Assurance
        \item DevOps/SysAdmin
        \item UX/UI Designer
        \item CTO/CIO
        \item Other
    \end{itemize}
    \item How many years of experience do you have participating in open source projects? *
    \begin{itemize}
        \item Less than 1 year
        \item 1-3 years
        \item 4-6 years
        \item 7-10 years
        \item More than 10 years
    \end{itemize}
    \item How many OSS projects have you participated in as a contributor? *
    \begin{itemize}
        \item 0-3
        \item 3-5
        \item 6-10
        \item 11-20
        \item More than 20
    \end{itemize}
    \item How often do you participate in code reviews in your capacity as maintainer? *
    \begin{itemize}
        \item More than once per day
        \item Daily
        \item Several times a week (less than once every day)
        \item Weekly
        \item Bi-Weekly
        \item Monthly
        \item Rarely (a few times per year)
        \item Never 
        \item Depends
    \end{itemize}
    \item Which sort of contributions do you make most frequently?
    \begin{itemize}
        \item Code Contributions
        \item Documentation
        \item Community Support
        \item Bug Reporting and Testing
        \item Design and UX
        \item Translation and Localization
        \item Other
    \end{itemize}
    \item In your opinion, what are the most important objectives of the code review process? [Reorder with 1 being highest importance]
    \item What do you believe are the key factors that ensure a contribution is approved during the code review process?
    \item Do you consult project documentation regarding the code review process for your contribution?
    \begin{itemize}
        \item Yes
        \item No
    \end{itemize}
    \item Which project specific documentation do you refer to get information on the code review process?
    \item Can you provide the link to these documents, if available?
    \item Please rate code review guideline documents in your project for the following (Strongly disagree to Strongly agree)
    \begin{itemize}
        \item Guidelines for the code review process are sufficiently documented.
        \item Documents are easily accessible to contributors.
        \item Documents clearly describe the exceptions expected from me while I perform my code review tasks.
        \item Documents have effectively addressed bias in the code review process.
        \item Documents have clearly defined the process to mitigate bias in the code review process.
        \item Documents have clearly defined the standard for communication during the code review process to minimize conflict.
        \item Objectives of the code review process as presented in these documentations are in line with my expectations for code review.
    \end{itemize}
    \item In your opinion, the current code review process (Strongly disagree to Strongly agree):
    \begin{itemize}
        \item Improves software quality.
        \item Effectively mitigates bias.
        \item Promotes diversity and inclusivity.
        \item Follows standards for communication during the code review process to minimize conflict.
    \end{itemize}
    \item Which of the following external resources do you consult about code reviews? (Check all that apply) 
    \begin{itemize}
        \item Guidelines documents from other projects/companies.
        \item Peer discussions.
        \item Online forums/blog posts.
        \item Training sessions.
        \item Other.
    \end{itemize}
    \item Have you ever noticed bias in the code review process?
    \begin{itemize}
        \item Yes
        \item No
    \end{itemize}
    \item If Yes, could you present the instance and how it was resolved?
    \item What are the challenges you face in implementing a code review process?
    \item What changes or improvements would you suggest for the code review process?
    \item Thank you for taking the time to complete our survey! Would you be open to participating in a follow-up interview to discuss your responses in greater detail? Please let us know if you’re interested and the best way to contact you. Are you willing to participate in a follow-up interview?
\begin{itemize}
\item Yes
\item No
\end{itemize}
\end{enumerate}
\section{Maintainer Survey Questions} \label{sec:maintainer_survey}
\textbf{Welcome to the Open Source Software (OSS) Code Review Process Survey}

\subsection*{Introduction}
Thank you for your interest in participating in this survey. Your input is invaluable in advancing our understanding of code review processes within Open Source Software (OSS) projects. This research aims to explore the intricacies and expectations of individuals like yourself who contribute to the rich ecosystem of OSS. In this survey, we use the term "code review" to refer to any of the following: "pull request review," "merge request review," or "change request review."

\subsection*{Purpose of the Study}
The core objective of this study is to delve into the code review mechanisms that are pivotal to the evolution and integrity of OSS. By gathering insights from both contributors and maintainers, we aim to paint a comprehensive picture of the current landscape, identify areas for improvement, and understand the tools and practices that can enhance the code review experience and mitigate biases. Bias in code review refers to the prejudicial treatment of contributions or contributors based on factors unrelated to the merit of the work, such as the contributor's identity, background, or the nature of the changes.

\subsection*{Who Should Participate}
Please note that to engage in this survey, participants are required to be aged 18 years or older. This survey is designed for:

\begin{itemize}
    \item \textbf{Maintainers}: Core team members who assess submitted code changes to decide on their incorporation into the project's code base.
\end{itemize}

Your experiences and perceptions as a contributor or maintainer are crucial in shaping the outcomes of this research.

\subsection*{What to Expect in This Survey}
The following areas will be covered in the survey:
\begin{itemize}
    \item Your role and experience in OSS projects.
    \item Expectations and experiences with the code review process.
    \item The use of tools, guidelines, or materials in facilitating code review.
    \item Perspectives on how code review processes can be improved to reduce bias.
\end{itemize}
In addition to demographic and background questions, there are 12 core questions in this survey, and we expect it to take about 10-12 minutes to complete.

\subsection*{Confidentiality}
Your responses will be kept confidential, and the data will be analyzed in aggregate form anonymously. However, we cannot protect the data to GDPR standards.

\subsection*{Consent}
Your participation in this survey is voluntary. If any question makes you feel uncomfortable, you can simply stop participating or close the browser window. You may decide not to participate at all, or, if you start the study, you may withdraw at any time. By proceeding with this survey, you acknowledge that you have read and understood the purpose of the research and agree to participate voluntarily.

\subsection*{Contact Information}
Should you have any questions or require further information about the study, please contact \textbf{\textit{<redacted for review>.}}

\subsection*{Start Survey}
To begin the survey, please click the "Start" button below. Thank you for your time and valuable contribution to this study.

\subsubsection*{Survey Questions}

\begin{enumerate}
    \item Please select your age group. *
    \begin{itemize}
        \item 18-24
        \item 25-34
        \item 35-44
        \item 45-54
        \item 55-64
        \item Above 64
    \end{itemize}
    \item Which of the following best describes your gender? *
    \begin{itemize}
        \item Male
        \item Female
        \item Non-binary/Third gender
        \item Prefer not to say
        \item Prefer to self-describe
    \end{itemize}
    \item What is the highest level of education you have completed?
    \begin{itemize}
        \item High school diploma or equivalent
        \item Some college, no degree
        \item Associate degree
        \item Bachelor’s degree
        \item Master’s degree
        \item Doctorate or higher
    \end{itemize}
    \item Please select the race/ethnicity group(s) with which you most closely identify. (Select all that apply) *
    \begin{itemize}
        \item Asian
        \item Black or African American
        \item Hispanic or Latino
        \item Native American or Alaska Native
        \item Native Hawaiian or Other Pacific Islander
        \item Middle Eastern or North African
        \item Multiracial
        \item White
        \item Prefer not to say
        \item Other (please specify)
    \end{itemize}
    \item How many years of professional experience do you have in software development? *
    \begin{itemize}
        \item Less than 1 year
        \item 1-3 years
        \item 4-6 years
        \item 7-10 years
        \item More than 10 years
    \end{itemize}
    \item What best describes your current role in the open source project? *
    \begin{itemize}
        \item Developer/Engineer
        \item Team Lead/Manager
        \item Quality Assurance
        \item DevOps/SysAdmin
        \item UX/UI Designer
        \item CTO/CIO
        \item Other
    \end{itemize}
    \item How many years of experience do you have participating in open source projects? *
    \begin{itemize}
        \item Less than 1 year
        \item 1-3 years
        \item 4-6 years
        \item 7-10 years
        \item More than 10 years
    \end{itemize}
    \item How many years of experience do you have participating in code reviews? *
    \begin{itemize}
        \item None
        \item Less than 1 year
        \item 1-3 years
        \item 4-6 years
        \item 7-10 years
        \item More than 10 years
    \end{itemize}
    \item How often do you participate in code reviews in your capacity as a maintainer? *
    \begin{itemize}
        \item More than once per day
        \item Daily
        \item Several times a week (less than once every day)
        \item Weekly
        \item Bi-Weekly
        \item Monthly
        \item Rarely (a few times per year)
        \item Never 
        \item Depends
    \end{itemize}
    \item What level of responsibility do you typically have as a reviewer in code reviews? *
    \begin{itemize}
        \item Primary decision-maker
        \item Shared decision-making
        \item Advisory role
        \item Observer
        \item Other
    \end{itemize}
    \item How many projects have you participated in as a maintainer/reviewer? *
    \begin{itemize}
        \item 0-3
        \item 3-5
        \item 6-10
        \item 11-20
        \item More than 20
    \end{itemize}
    \item In your role as a code maintainer, rank your primary responsibilities in the order of importance.
    \begin{itemize}
        \item Finalizing code decisions
        \item Ensuring code quality and standards
        \item Managing codebase and documentation
        \item Overseeing project direction
        \item Mentoring or guiding contributors
        \item Other
    \end{itemize}
    \item In your opinion, what are the most important objectives of the code review process? [Reorder with 1 being highest importance]
    \item What do you believe are the key factors that ensure a contribution is approved during the code review process?
    \item Do you consult project documentation regarding the code review process for your code reviews? *
    \begin{itemize}
        \item Yes
        \item No
    \end{itemize}
    \item Which project-specific documentation do you refer to get information on the code review process?
    \item Can you provide the link to these documents, if available?
    \item Please rate code review guideline documents in your project for the following (Strongly disagree to Strongly agree):
    \begin{itemize}
        \item Guidelines for the code review process are sufficiently documented.
        \item Documents are easily accessible to contributors.
        \item Documents clearly describe the expectations from me while I perform my code review tasks.
        \item Documents have effectively addressed bias in the code review process.
        \item Documents have clearly defined the process to mitigate bias in the code review process.
        \item Documents have clearly defined the standard for communication during the code review process to minimize conflict.
        \item Objectives of the code review process as presented in these documentations are in line with my expectations for code review.
    \end{itemize}
    \item In your opinion, the current code review process (Strongly disagree to Strongly agree):
    \begin{itemize}
        \item Improves software quality
        \item Effectively mitigates bias
        \item Promotes diversity and inclusivity
        \item Follows standards for communication during the code review process to minimize conflict
    \end{itemize}
    \item Which of the following external resources do you consult about code reviews? (Check all that apply) 
\begin{itemize}
    \item Guidelines documents from other projects/companies
    \item Peer discussions
    \item Online forums/blog posts
    \item Training sessions
    \item Other
\end{itemize}
\item Have you ever noticed bias in the code review process? *
\begin{itemize}
    \item Yes
    \item No
\end{itemize}
\item If Yes, could you present the instance and how it was resolved?
\item What are the challenges you face in implementing a code review process?
\item What changes or improvements would you suggest for the code review process?
\item Thank you for taking the time to complete our survey! Would you be open to participating in a follow-up interview to discuss your responses in greater detail? Please let us know if you're interested and the best way to contact you. Are you willing to participate in a follow-up interview?
\begin{itemize}
    \item Yes
    \item No
\end{itemize}
\end{enumerate}
